# Supplementary material for: Control VAR: a counterfactual based approach to inference in macroeconomics
Source: arXiv:2510.23762 source file (2026-10-24)
Supplement: Supplementary file 1 [file tab_california_appendix.tex]

\begin{table}[htbp]
\centering
\caption{Pass-through of the LCFS cost: lag orders}
\label{tab:california_appendix}
\small
\begin{tabular}{lccccc}
\toprule
 & Lags & Impact & 1 month & 12 months & Width ratio \\
\midrule
\multicolumn{6}{l}{Lag order (both models)} \\
\midrule
Gulf Coast (PADD 3), lag order 1 & 1/1 & 1.20$^{\dagger}$ & 1.97$^{*}$ & 1.98$^{*}$ & 0.55 \\
\footnotesize  &  & [-0.03, 2.71] & [0.04, 4.28] & [0.02, 4.48] &  \\[2pt]
Gulf Coast (PADD 3), lag order 2 & 2/2 & 1.06$^{\dagger}$ & 1.52$^{\dagger}$ & 0.76 & 0.54 \\
\footnotesize  &  & [-0.26, 2.60] & [-0.71, 3.83] & [-1.10, 2.96] &  \\[2pt]
Gulf Coast (PADD 3), lag order 4 & 4/4 & 0.99$^{\dagger}$ & 1.55$^{\dagger}$ & 0.88 & 0.43 \\
\footnotesize  &  & [-0.24, 2.40] & [-0.39, 3.56] & [-1.32, 3.14] &  \\[2pt]
Gulf Coast (PADD 3), lag order 6 & 6/6 & 1.01$^{\dagger}$ & 1.54$^{\dagger}$ & 1.15 & 0.40 \\
\footnotesize  &  & [-0.11, 2.54] & [-0.38, 3.75] & [-1.40, 4.18] &  \\[2pt]
Gulf Coast (PADD 3), lag order 8 & 8/8 & 1.00$^{\dagger}$ & 1.41$^{\dagger}$ & 0.93 & 0.37 \\
\footnotesize  &  & [-0.33, 2.55] & [-1.00, 3.58] & [-1.95, 3.46] &  \\[2pt]
Gulf Coast (PADD 3), lag order 12 & 12/12 & 1.07$^{\dagger}$ & 1.46$^{\dagger}$ & -0.00 & 0.38 \\
\footnotesize  &  & [-0.39, 2.85] & [-0.64, 3.99] & [-3.10, 3.43] &  \\[2pt]
PADDs 1 to 4, lag order 1 & 1/1 & 0.82$^{\dagger}$ & 1.85$^{*}$ & 1.84$^{*}$ & 0.49 \\
\footnotesize  &  & [-0.34, 2.43] & [0.03, 3.99] & [0.06, 4.01] &  \\[2pt]
PADDs 1 to 4, lag order 2 & 2/2 & 0.77 & 1.55$^{\dagger}$ & 0.88 & 0.55 \\
\footnotesize  &  & [-0.59, 2.39] & [-0.47, 3.88] & [-0.92, 3.19] &  \\[2pt]
PADDs 1 to 4, lag order 4 & 4/4 & 0.65 & 1.59$^{\dagger}$ & 0.87 & 0.40 \\
\footnotesize  &  & [-0.56, 1.95] & [-0.17, 3.51] & [-1.15, 2.92] &  \\[2pt]
PADDs 1 to 4, lag order 6 & 6/6 & 0.66$^{\dagger}$ & 1.64$^{\dagger}$ & 1.39 & 0.40 \\
\footnotesize  &  & [-0.43, 2.12] & [-0.23, 3.66] & [-1.13, 4.31] &  \\[2pt]
PADDs 1 to 4, lag order 8 & 8/8 & 0.67 & 1.53$^{\dagger}$ & 1.08 & 0.34 \\
\footnotesize  &  & [-0.57, 2.06] & [-0.45, 3.41] & [-1.54, 3.56] &  \\[2pt]
PADDs 1 to 4, lag order 12 & 12/12 & 0.69 & 1.57$^{\dagger}$ & 0.47 & 0.38 \\
\footnotesize  &  & [-0.76, 2.29] & [-0.45, 3.99] & [-2.63, 3.93] &  \\[2pt]
\bottomrule
\end{tabular}
\begin{minipage}{0.95\textwidth}\footnotesize
Note: cumulated response of the California retail price, in cents per gallon, to an increase of 1 cent per gallon in the LCFS cost, from the CVAR in the differenced branch with equal weights on the controls. Policy: the cost per gallon implied by the CARB formula before May 2024 and the cost reported by refiners to the California Energy Commission from then on, in monthly changes, unless stated otherwise. Lags: CVAR / VAR without controls. 90 percent residual bootstrap bands in brackets; $^{\dagger}$ the 68 percent band excludes zero; $^{*}$ the 90 percent band excludes zero. Width ratio: width of the CVAR band over that of the VAR without controls, at 12 months.
\end{minipage}
\end{table}
